# Supplementary material for: Homogeneous Dynamics Space for Heterogeneous Humans
Source: arXiv:2412.06146 source file (2025-03-14)
Supplement: Supplementary file 1 [file suppl.tex]

   % CVPR 2024 Paper Template; see https://github.com/cvpr-org/author-kit

\documentclass[10pt,twocolumn,letterpaper]{article}

%%%%%%%%% PAPER TYPE  - PLEASE UPDATE FOR FINAL VERSION
\usepackage{cvpr}              % To produce the CAMERA-READY version
% \usepackage[review]{cvpr}      % To produce the REVIEW version
% \usepackage[pagenumbers]{cvpr} % To force page numbers, e.g. for an arXiv version

% Import additional packages in the preamble file, before hyperref
\input{preamble}

% It is strongly recommended to use hyperref, especially for the review version.
% hyperref with option pagebackref eases the reviewers' job.
% Please disable hyperref *only* if you encounter grave issues, 
% e.g. with the file validation for the camera-ready version.
%
% If you comment hyperref and then uncomment it, you should delete *.aux before re-running LaTeX.
% (Or just hit 'q' on the first LaTeX run, let it finish, and you should be clear).
\definecolor{cvprblue}{rgb}{0.21,0.49,0.74}
\usepackage[pagebackref,breaklinks,colorlinks,citecolor=cvprblue]{hyperref}

\newcommand*\samethankss[1][\value{footnote}]{\footnotemark[#1]}
%%%%%%%%% PAPER ID  - PLEASE UPDATE
 % *** Enter the Paper ID here todo

%%%%%%%%% TITLE - PLEASE UPDATE
\title{Supplementary Materials for ``Homogeneous Dynamics Space for Heterogeneous Humans''}

%%%%%%%%% AUTHORS - PLEASE UPDATE
\author{
Xinpeng Liu$^{1,2}$,~
Junxuan Liang$^1$,~
Chenshuo Zhang$^1$,~
Zixuan Cai$^3$,~
Cewu Lu$^{1,2}$\thanks{Corresponding authors.},~
Yong-Lu Li$^{1,2}$\samethankss~\\
\tt\small{$^1$Shanghai Jiao Tong University}, \tt\small{$^2$Shanghai Innovation Institute}, \tt\small{$^3$Soochow University}\\
\tt\small{xinpengliu0907@gmail.com}, \tt\small{zxcai@stu.suda.edu.cn}, \\
\tt\small{\{whitefork, zhangchenshuo, lucewu, yonglu\_li\}@sjtu.edu.cn}\\
}

\begin{document}
\maketitle
\input{sec/6-appendix}

% \newpage
{
    \small
    \bibliographystyle{ieeenat_fullname}
    \bibliography{ref}
}

% WARNING: do not forget to delete the supplementary pages from your submission 
% \input{sec/6-appendix}

\end{document}
